# Supplementary material for: Mitigating Data Reconstruction Attacks in Federated Learning: Conditions, Bounds, and Theoretical Guarantees
Source: arXiv:2407.16735 source file (2026-10-17)
Supplement: Supplementary file 1 [file Appendix_4.tex]

\textcolor{blue}{
\section{Design of Prompts for the InferDPT Framework}\label{prompt}
Since our methods for quantifying privacy leakage and utility loss differ, we designed distinct prompts for each.
\subsection{Prompts for Quantifying Privacy Leakage}
For quantifying privacy leakage, we only used the black-box LLM for inference. The prompt we used is as follows:}

\textcolor{blue}{
\textit{
To quantify privacy leakage, we used only the black-box LLM for inference. The prompt we employed is as follows:}}

\textcolor{blue}{
\textit{
there are some examples:}}

\textcolor{blue}{
\textit{
    Original: The company announced record profits in the third quarter.
    Perturbed: Business speak happy money three time part.
    Recovered: The business reported positive financial results in the third period.}}

\textcolor{blue}{
\textit{
    Original: Scientists discover new species in Amazon rainforest.
    Perturbed: People find thing green tree place.
    Recovered: Researchers identified a new organism in the tropical forest.}}

\textcolor{blue}{
\textit{
        ——Perturbed:  }}

\textcolor{blue}{
\textit{
       You should only respond the recovered tokens.}}
       
\textcolor{blue}{
\textit{
       ——Output format:
       [token1] [token2] [token3] ...}}

\textcolor{blue}{
\subsection{Prompts for Quantifying Utility Loss}}
\textcolor{blue}{For evaluating utility loss, we used both the black-box LLM and the local LLM for inference. Given that the tasks for these two LLMs are different, we created separate prompts for each, as follows:}

\textcolor{blue}{
\textbf{Prompt for Black-box LLM:}}

\textcolor{blue}{
\textit{
You are a creative writer skilled in continuing stories and texts in a natural and engaging way.Your task is to generate a coherent continuation that matches the style and context of the original text.}}

\textcolor{blue}{
\textit{
Continue this text in a natural and engaging way, maintaining the same style and tone. Write 2-3 sentences that flow naturally from the original text.}}

\textcolor{blue}{
\textit{
——Original Text: }}

\textcolor{blue}{
\textit{
——[your continuation]}}

\textcolor{blue}{
\textbf{Prompt for Local LLM:}}

\textcolor{blue}{
\textit{
Analyze the coherence between the "Prefix Text" and "Perturbed Generation", then follow these rules:}}

\textcolor{blue}{
\textit{
        1. If the "Perturbed Generation" meets ALL these criteria:}}

\textcolor{blue}{
\textit{
           - Continues the story/topic from the "Prefix Text" naturally}}

\textcolor{blue}{
\textit{
           - Maintains consistent facts and details}}
           
\textcolor{blue}{
\textit{
           - Uses similar tone and style}}
           
\textcolor{blue}{
\textit{
           → Output the "Perturbed Generation" exactly as is}}
           
\textcolor{blue}{
\textit{
        2. Otherwise, if ANY criteria are not met:}}
        
\textcolor{blue}{
\textit{
           - Write a new continuation that:}}
           
\textcolor{blue}{
\textit{
           - Directly follows from the last sentence of "Prefix Text"}}
           
\textcolor{blue}{
\textit{
           - Matches the style and tone of "Perturbed Generation"}}
           
\textcolor{blue}{
\textit{
           - Maintains factual consistency with "Prefix Text"}}
           
\textcolor{blue}{
\textit{
        OUTPUT ONLY the continuation text, with no explanations or additional text.}}
        

\textcolor{blue}{
\textit{
        ——"Prefix Text": }}
        
\textcolor{blue}{
\textit{
        ——"Perturbed Generation": }}
        
\textcolor{blue}{
\textit{
        ——"Your Continuation":}}
